# Supplementary material for: Synthesize Dexterous Nonprehensile Pregrasp for Ungraspable Objects
Source: arXiv:2305.04654 source file (2023-05-08)
Supplement: Supplementary file 1 [file appendix.tex]

\appendix
